# Supplementary material for: WordRobe: Text-Guided Generation of Textured 3D Garments
Source: arXiv:2403.17541 source file (2024-07-14)
Supplement: Supplementary file 1 [file X_suppl.tex]

\clearpage
\setcounter{page}{1}
\maketitlesupplementary
 
% \section{Background}
\section{Text-driven Garment Editing}
In this section, we describe how to enable text-driven editing of garments. Given a garment latent code $\phi$, methods like \cite{de2023drapenet} employ a pretrained latent code classifier to identify the garment type and to identify which dimension to interpolate in order to induce category-specific changes, e.g. manipulate sleeve lengths. Though this approach works well, it requires explicit manual annotations to enable control over interpolation. In our case, we make use of CLIP embeddings to automatically identify the dimensions to control certain aspects of the 3D garment. Given a CLIP embedding $\psi$ corresponding to a text-prompt (say, \textit{``skirt''}), $MLP_Map$ predicts corresponding garment latent code $\phi$ which is decoded to obtain the initial garment. For a text prompt \textit{``long''} we first compute the CLIP embedding $\psi_{feature}$. Then, we perform the following operation: 
\begin{equation}
    \psi_{edit} = w\psi + (1-w)\psi_{feature}
\end{equation}
\noindent
In other words, we perturb the $\psi$ in the direction of $\psi_{feature}$ ($w=0.5$), which results in the modified CLIP embedding $\psi_{edit}$. $MLP_{map}$ takes this $\psi_{edit}$ and predicts $\phi_{mod}$, which if decoded results in the 3D garment which resembles \textit{``long skirt''}. However, predicting the entire garment latent code from scratch disturbs other characteristics of the original garment as well. To retain the other characteristics and change only the \textit{length}, we first compute the difference $\phi_{delta}$ between original latent code $\phi$ and modified latent code $\phi$, i.e. $\phi_{delta}=\phi - \phi_{mod}$. We then identify top-$k$ values in $\phi_{delta}$, which denote the corresponding dimensions to change in order to achieve the desired modification. Thus, perturbing the garment latent code $\phi$ along only these $k$ dimensions results in intended modification, while maintaining other characteristics of the garment (choosing the value of k is flexible and is driven by the user preference, we use $k=7$). We perform text-driven editing of \textit{\textbf{``skirt''}} according to the keyword \textit{``long''} (\autoref{fig:editing}(a)), and that of a \textit{\textbf{``cardigan"}} (\autoref{fig:editing}(b)) by introducing \textit{``sleeves''} and then \textit{``hood''}. This approach does not require any manual intervention, except the amount of perturbation the end-user intends to introduce.

\begin{figure*} 
    \centering
    \includegraphics[width=\linewidth]{figures/editing.pdf}
    \caption{Text-driven editing of 3D garments.}
    \label{fig:editing}
\end{figure*}

\section{Extended Evaluation}
\subsection{Comparison with Text-to-3D Methods}
We compare the quality of generated garments from WordRobe with existing state-of-the-art text-to-3D generative methods $-$ Shap-E \cite{jun2023shape} \& ProlificDreamer \cite{wang2023prolificdreamer} in \autoref{fig:text_to_3d}. Both of these methods are generic text-to-3D methods, trained on millions of training samples, inheriting zero-shot generation capabilities. However, their output geometry quality is not sufficient to be directly integrated into a standard graphics pipeline. Moreover, they don't offer interpolation for controllable generation/editing. Specifically, \cite{wang2023prolificdreamer} follows an optimization-based framework, resulting in a very slow generation process (approx $1.5$ hours on an NVIDIA RTX 4090 GPU). \cite{jun2023shape} demonstrates faster processing times (approx. 10 seconds) due to its efficient representation. However, it operates on a lower resolution volume grid of 128, significantly inferior compared to WordRobe, which provides an $4$ times better resolution (grid-size$=512$) over \cite{jun2023shape}. Despite the enhanced resolution, our method requires only about 40 seconds for end-to-end garment generation ($18$ sec. for geometry synthesis $+$ $22$ sec. for texture synthesis). \textbf{\textit{Please refer to the supplementary video to better appreciate the quality difference between the aforementioned methods and our proposed method.}}
\begin{figure}
    \centering
    \includegraphics[width=\linewidth]{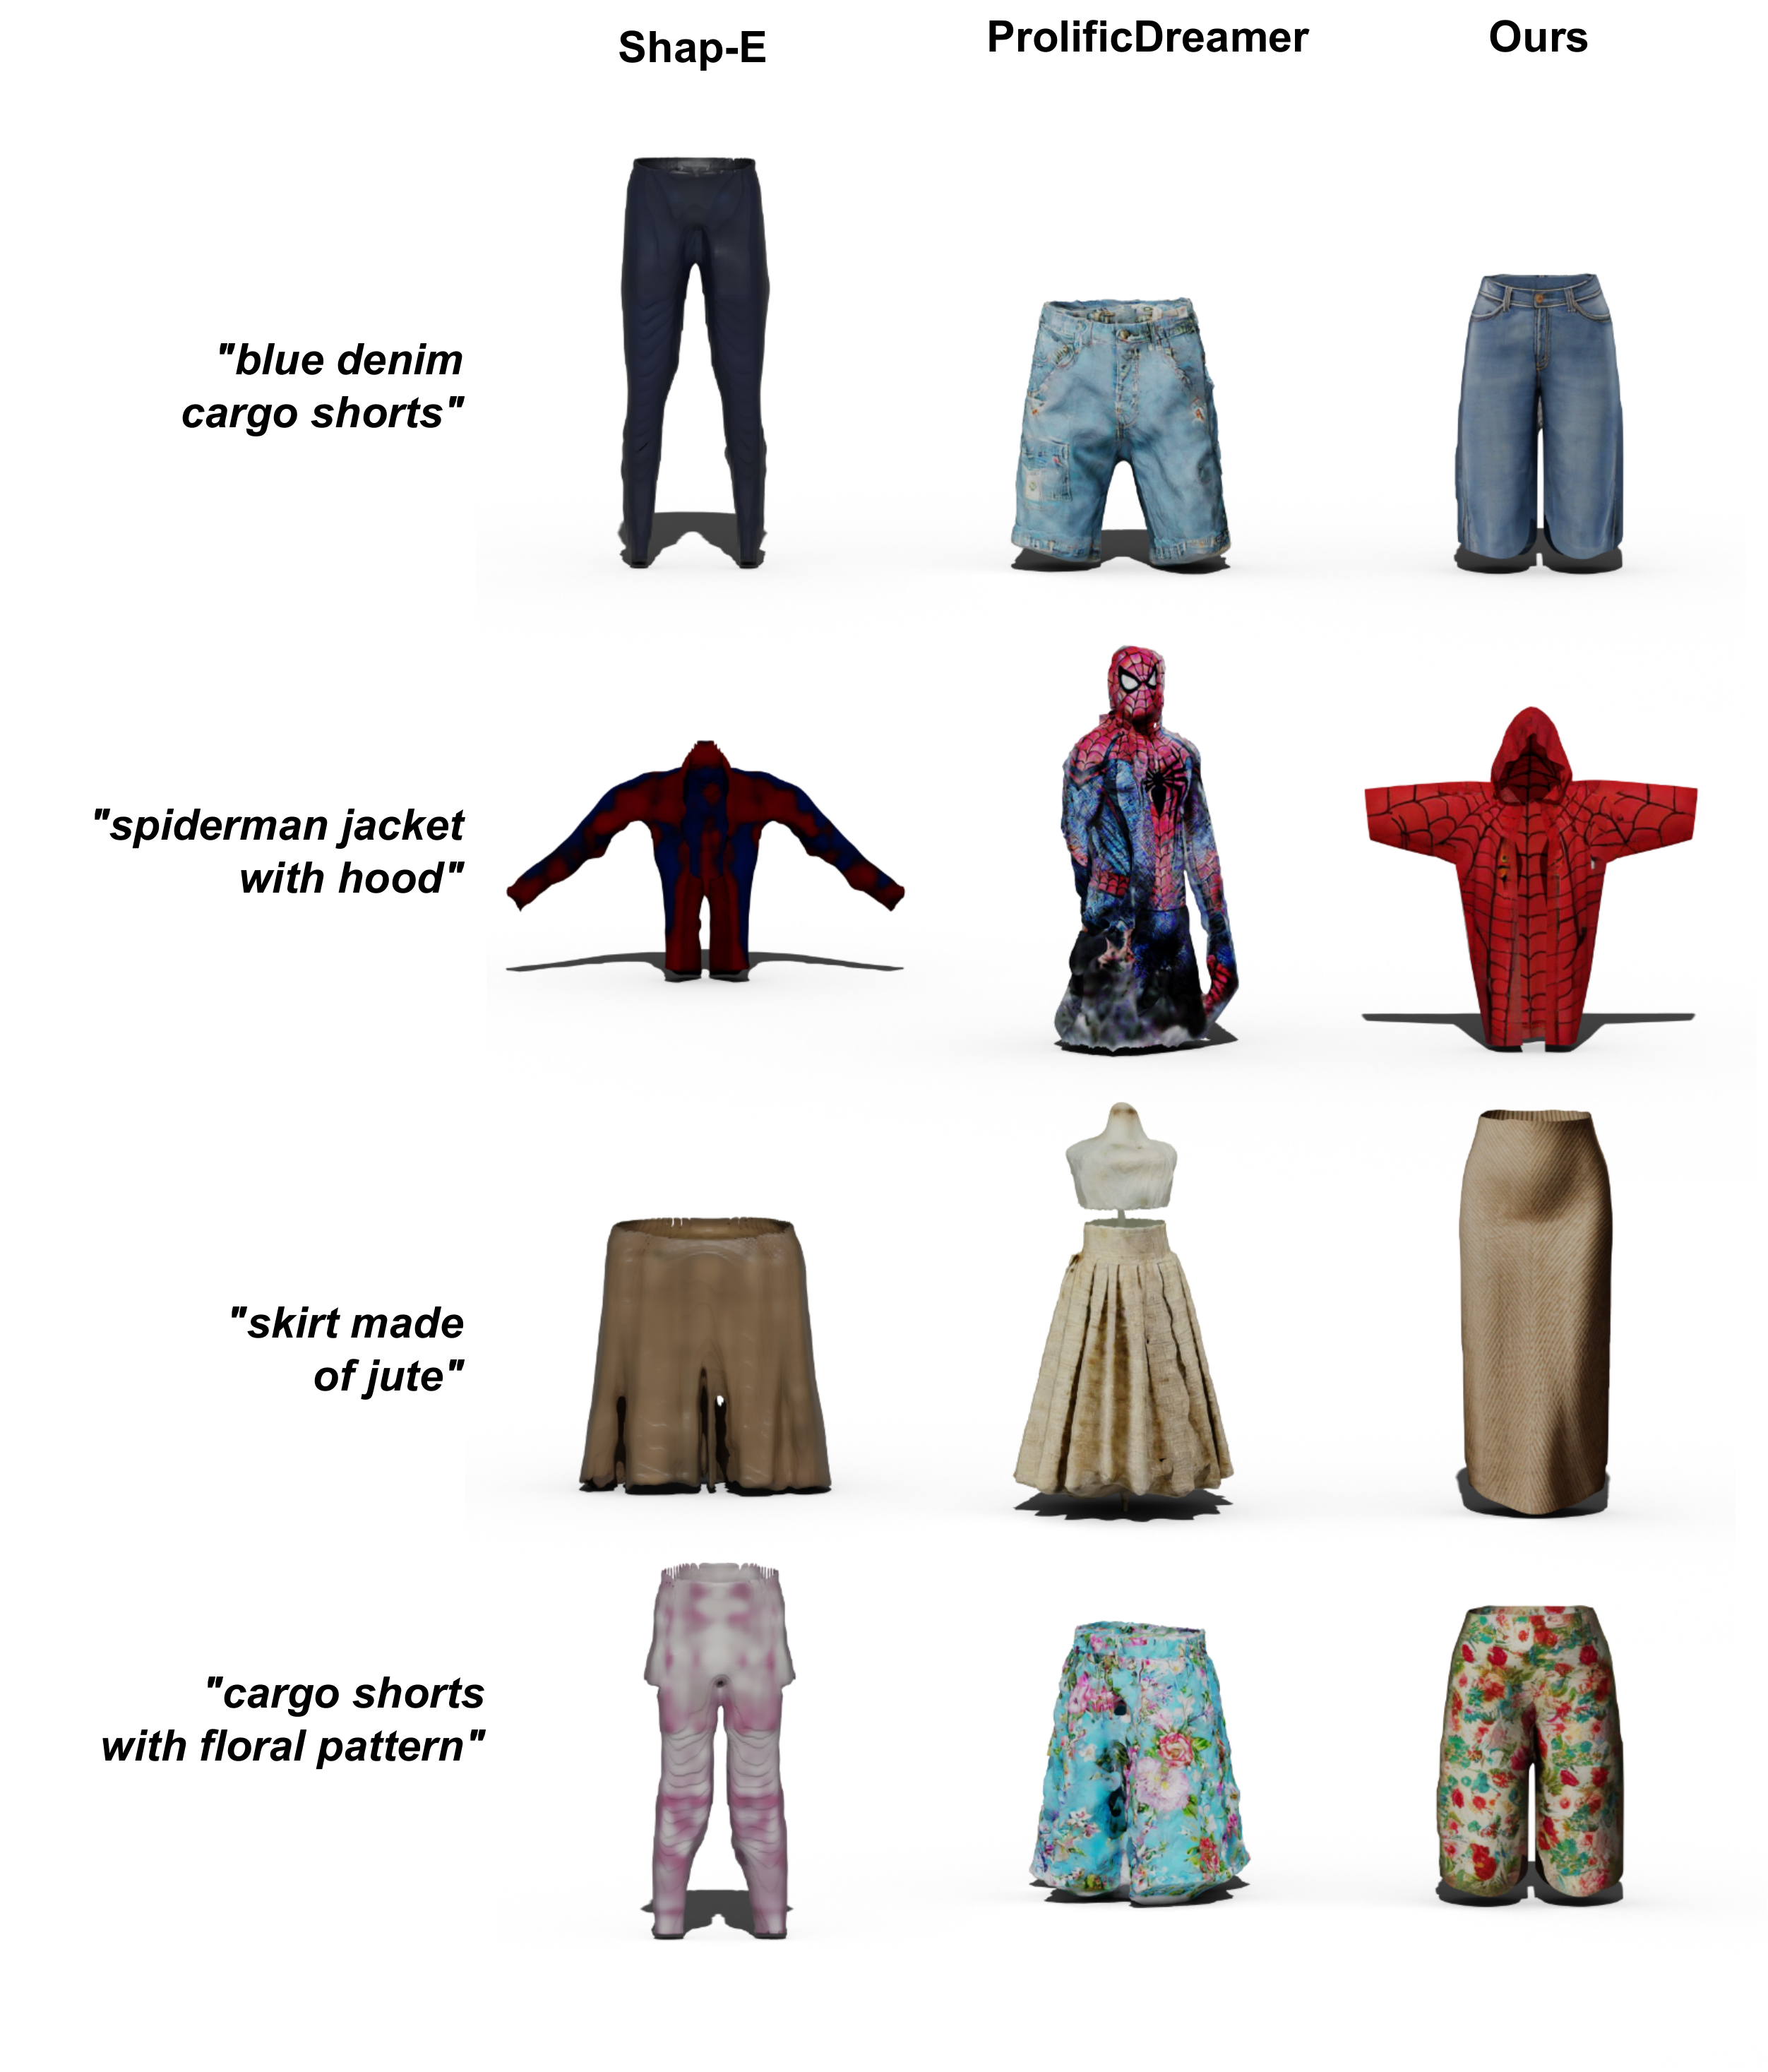}
    \caption{Qualitative comparison with Text-to-3D SOTA methods.}
    \label{fig:text_to_3d}
\end{figure}

\subsection{User Study}
For the subjective evaluation of our method, we perform a qualitative user study among $67$ participants. First, the participants were presented with the results of our method and were ask two questions :
\begin{itemize}
    \item \textit{\textbf{How would you rate the relationship between the input text prompt and the generated result on a scale of 1 to 3? [1-not related, 2-somewhat related, 3-highly related]}}
    \item \textit{\textbf{How would you rate the quality of the results in general, on a scale of 1 to 5? [1-very bad, 2-bad, 3-acceptable, 4-good, 5-very good]}}
\end{itemize}

Our method achieves an average rating of $\mathbf{2.57}$ on a scale of $[1-3]$ in terms of the relationship between the result and the input text prompt, and an average rating of $\mathbf{4.01}$ on a scale of $[1-5]$ in terms of quality of the generated 3D garment.

All the participants were also asked to select one of the methods among \cite{jun2023shape}, \cite{wang2023prolificdreamer} and WordRobe on two basis $-$ relationship between the result \& text-prompt, and overall quality of the generated garment. About $63\%$ of the participants prefer WordRobe, $27\%$ prefer \cite{wang2023prolificdreamer}, and $10\%$ prefer \cite{jun2023shape} in terms of relationship between the result and text prompt. In terms of quality, $65\%$ of the participants prefer WordRobe, $28\%$ prefer \cite{wang2023prolificdreamer}, and $7\%$ prefer \cite{jun2023shape}.

Finally, we also asked participants to choose between Text2Tex\cite{chen2023text2tex} and WordRobe for the text-driven synthesis of textures over existing meshes. About $54\%$ participants opted for WordRobe when it comes to the relationship between the result and input text prompt, and about $76\%$ opted for WordRobe when it comes to the quality of the generated 3D garment.
% \section{Discussion}
\section{Limitations}
\begin{figure}
    \centering
    \includegraphics[width=\linewidth]{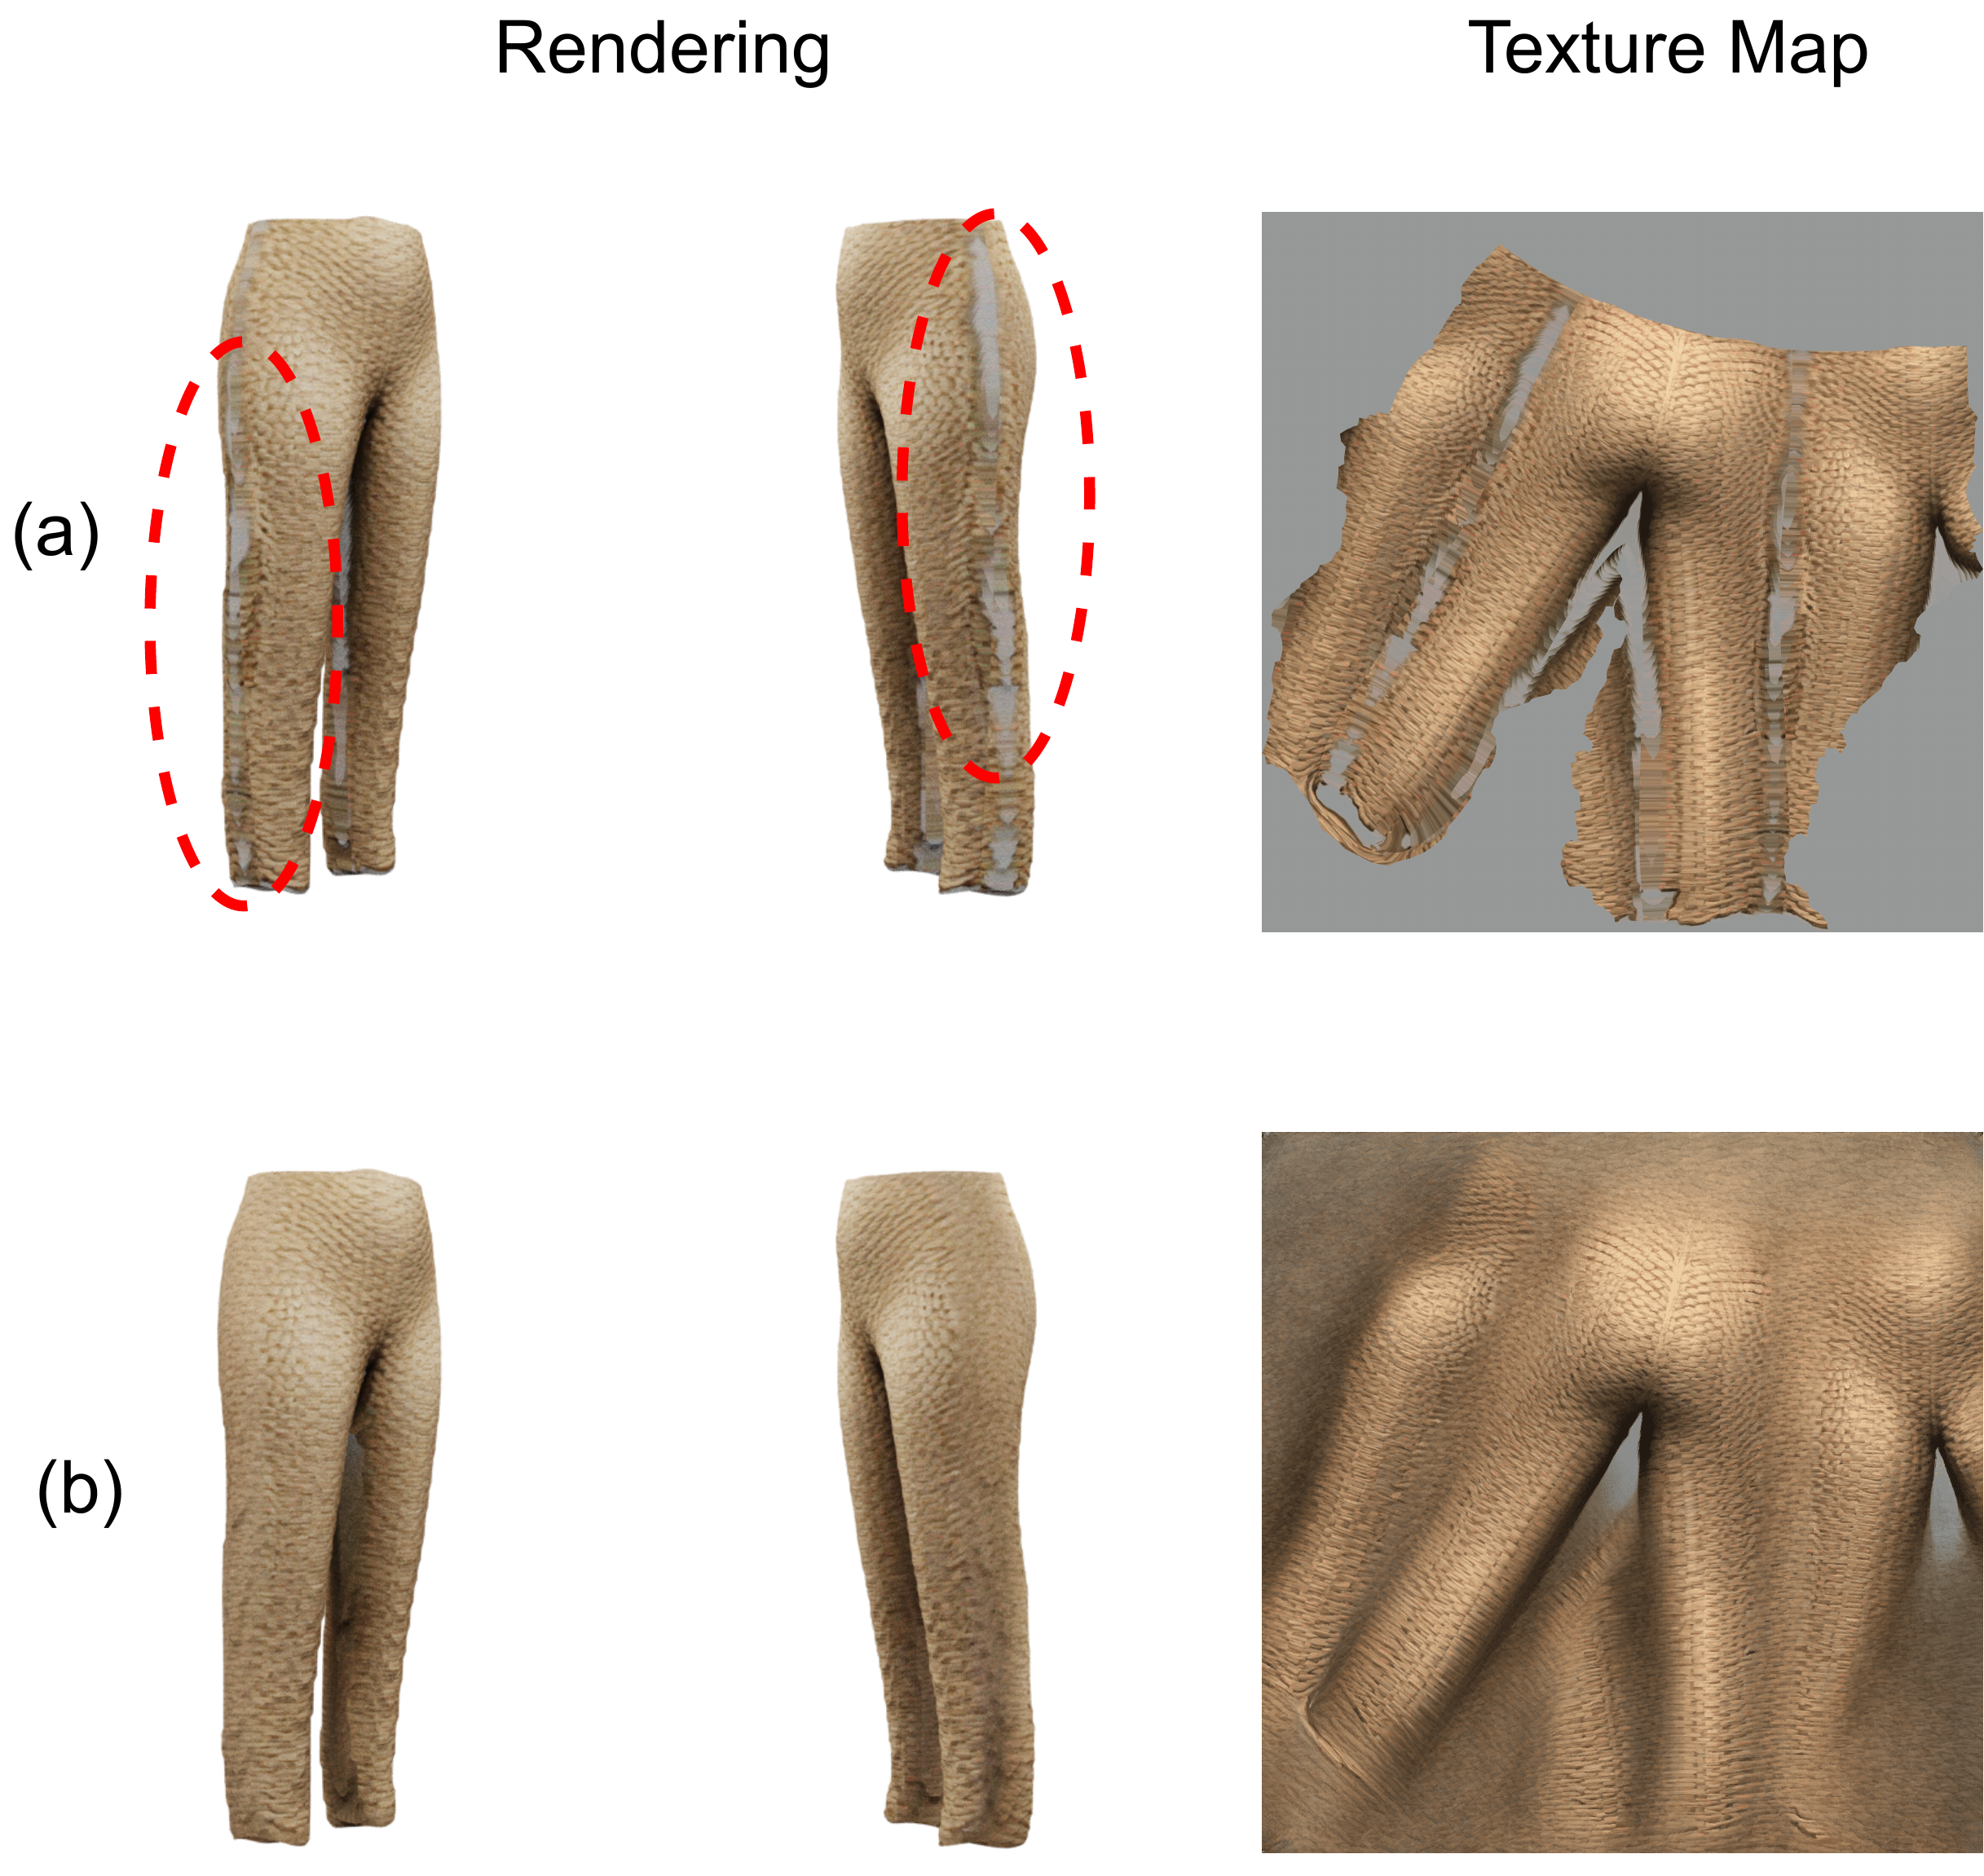}
    \caption{(a) Missing tangential information due to orthographic projection. (b) Details inpainted within the texture map.}
    \label{fig:inpaint}
\end{figure}
WordRobe generates high-fidelity 3D garments with high-quality textures at an unprecedented speed and scale. However, there are certain limitations to our approach that we wish to overcome in the future. One of the drawbacks of front-back orthographic rendering is the loss of information around the tangential regions (see \autoref{fig:inpaint}). In order to fill in the missing details, we employ an off-the-shelf inpainting method which occasionally leaves blurry seams along the boundary of the front \& back regions. Another limitation is the lack of fine-grain garment parts, e.g. pockets, buttons, etc. which are challenging to model using implicit representations such as UDF.

In the context of text-driven texture synthesis, one major limitation that every existing method encounters is the hallucination of shadows, lights, and edges which are purely textural and not a part of the surface of the garment. Though it may enhance the garment's appearance, from the graphics application point of view, this is an inconvenience. As a part of future work, we wish to explore relighting to get rid of false shading, retaining the true albedo of the garment geometry. We also like to enable support for layered clothing and material property of the garments. We hope our work paves a path towards high-fidelity production-ready garment generation from natural language prompts.
